# Supplementary material for: Entailment Semantics Can Be Extracted from an Ideal Language Model
Source: arXiv:2209.12407 source file (2024-01-08)
Supplement: Supplementary file 2 [file old-appendices.tex]

\section{Independently Truthful Speakers} \label{sec:ind-truthful}

After establishing an isomorphism results for uniformly truthful speakers in \autoref{sec:uniform-true}, we will now generalize the proof to hold for a broader class of slightly more natural speakers. Intuitively, the class of speakers we will introduce in this section always tell the truth, but, unlike uniformly truthful speakers, can assign different probabilities to different true sentences. We will also enforce conditional independence of different sentences given the world $w$. Therefore, we refer to such speakers as independently truthful.

\subsection{Definition}

We formalize a class of speakers who never lie, and where different sentences are conditionally independent given the world. In other words, the probability of a sentence $y$ cannot depend on a previous sentence $x$ in the same text, besides the fact that they come from the same world.

\begin{definition}
A speaker is \emph{independently truthful} if they satisfy:
\begin{itemize}
    \item \textbf{Conditional independence:} For all worlds $w \in \mathcal W$ and sentences $x, y \in \mathcal X$,
    \begin{equation*}
        p(y \mid x, w) = p(y \mid w) .
    \end{equation*}
    This property is illustrated in \autoref{fig:indep}.
    \item \textbf{Factorized truthfulness:} There exist functions $f : \mathcal X \to \mathbb{R}^+$ and $g: \mathcal W \to \mathbb{R}^+$ such that, for all sentences $x$,
    \begin{equation*}
        p(x \mid w) = \den{x}(w) f(x) g(w) . 
    \end{equation*}
\end{itemize}
\end{definition}

Natural language speakers clearly violate conditional independence, since speakers explicitly seek to avoid reproducing redundant information, implying that $y$ depends on $x$. Rather, the assumption is a useful starting point that aids the analysis. Later in \autoref{sec:informative}, we will relax this simplifying assumption and examine the implications for the isomorphism between form and meaning.

The factorized truthfulness assumption, on the other hand, is not problematic. It is general enough to express a variant of rational speakers under the Rational Speech Acts \citep[RSA;][]{goodman2016pragmatic} framework where speakers are constrained to be conditionally independent (see \autoref{sec:rsa}). RSA is a formal model of linguistic pragmatics where speakers optimize the amount of information their utterance conveys to their imagined listener.
With conditional independence, this means that sentences are weighted by the amount of information they convey about $w$.
Thus, independently truthful speakers can be somewhat informative to their listeners, but a full text of several sentences is not maximally informative, since later sentences will be unnaturally redundant with earlier ones.

\begin{figure}
    \centering
    % \begin{subfigure}
    \begin{tikzpicture}
    \node[state,fill={rgb:red,1;green,2;blue,5}] (w) {\textcolor{white}{$w$}};
    \node[state,below left of=w] (x) {$x$};
    \node[state,below right of=w] (y) {$y$};
    % \node[draw=black,fit=(w) (x) (y), inner sep=0.2cm] (speaker) {};
    % \node[state,below of=speaker,pattern=dots] (p) at (0, -1) {$p(xy)$};
    \path (w) edge (x);
    \path (w) edge (y);
    \path (x) edge (y);
    % \path (x) edge (p);
    % \path (y) edge (p);
    \end{tikzpicture}
    % \end{subfigure}
    % \begin{subfigure}
    \qquad \qquad \qquad
    \begin{tikzpicture}
    \node[state,fill={rgb:red,1;green,2;blue,5}] (w) {\textcolor{white}{$w$}};
    \node[state,below left of=w] (x) {$x$};
    \node[state,below right of=w] (y) {$y$};
    % \node[draw=black,fit=(w) (x) (y), inner sep=0.2cm] (speaker) {};
    % \node[state,below of=speaker,pattern=dots] (p) at (0, -1) {$p(xy)$};
    \path (w) edge (x);
    \path (w) edge (y);
    % \path (x) edge (p);
    % \path (y) edge (p);
    \end{tikzpicture}
    % \end{subfigure}
    \caption{Causal diagram for dataset generation without conditional independence (left) and with it (right). The relationship between $w$ and $x$ is specified by a speaker $p(x \mid w)$ (and analogously for $y$). The world $w$ is latent, so the target distribution for a LM is the marginal distribution $p(xy)$.}
    \label{fig:indep}
\end{figure}

\subsection{Results}

We will show that, assuming speakers are independently truthful, entailment is isomorphic to a distributional relation.
Define a tautology $\tau \in \mathcal X$ as a sentence that is true in every world, i.e., $\den{\tau} = \mathcal W$.

\begin{theorem} \label{thm:cia-sta}
Under any independently truthful speaker $p$ and any tautology $\tau$, entailment is isomorphic to a distribution relation $d_{p,\tau}(x, y)$. Specifically, for any sentences $x,y \in \mathcal X$,
\begin{equation*}
    \den{x} \subseteq \den{y} \iff \frac{p(xy)}{p(y\tau)} = \frac{p(xx)}{p(x\tau)} .
\end{equation*}
\end{theorem}
\begin{proof}
Applying conditional independence, we write $p(xy)$ as
\begin{align*}
    p(xy)
    &= \sum_w p(x \mid w) p(y \mid x, w) p(w) \\
    &= \sum_w p(x \mid w) p(y \mid w) p(w)
     .
\end{align*}
Next, we leverage factorized truthfulness to expand this as
\begin{align*}
    p(xy)
    &= \sum_w \den{x}(w) f(x) g(w) \den{y}(w) f(y) g(w) p(w) \\
    &= f(x) f(y) \sum_w \den{x}(w) \den{y}(w) p(w) g(w)^2 \\
    &= f(x) f(y) \sum_w \den{x}(w) \den{y}(w) c(w) ,
\end{align*}
where we let $c(w) \triangleq p(w) g(w)^2$ as a convenient shorthand.
For any tautology $\tau$, we can derive that
\begin{align*}
    \frac{p(x\tau)}{p(xx)}
        = \frac{f(x)f(\tau)\sum_w \den{x}(w) c(w)}{f(x)^2 \sum_w \den{x}(w) c(w)}
        = \frac{f(\tau)}{f(x)} .
\end{align*}
As a result, $p(x\tau)$ and $p(y\tau)$ have the result of ``normalizing'' the left and right-hand sides of the proposed distributional relation $d_{p,\tau}(x, y)$:
\begin{align*}
    \frac{p(xy)}{p(y\tau)} &= \frac{f(x)}{f(\tau)} \sum_w \den{x}(w) \den{y}(w) c(w) \\
    \frac{p(xx)}{p(x\tau)} &= \frac{f(x)}{f(\tau)} \sum_w \den{x}(w) c(w) .
\end{align*}
Cancelling $\frac{f(x)}{f(\tau)}$ on each side, we can invoke \autoref{lem:sum-entails} to conclude that $d_{p,\tau}(x, y)$ holds if and only if, for all $w$, $\den{x}(w) \den{y}(w) = \den{y}(w)$. We conclude that $d_{p,\tau}(x, y)$ holds if and only if $\den{x} \subseteq \den{y}$.
\end{proof}

Since the empty string $\omega$ is a tautology, and $p(x) = 2p(x \omega)$ by conditional independence, we immediately obtain:

\begin{corollary} \label{cor:sta-cia}
Under any independently truthful speaker $p$, entailment is isomorphic to a distributional relation. Specifically, for any sentences $x,y \in \mathcal X$,
\begin{equation*}
    \den{x} \subseteq \den{y} \iff \frac{p(xy)}{p(y)} = \frac{p(xx)}{p(x)} .
\end{equation*}
\end{corollary}

\subsection{Discussion}
In \autoref{cor:sta-cia}, we have derived a distributional relation isomorphic to entailment that holds under any independently truthful speaker.
This is much more general than the result in \autoref{sec:uniform-true}, as independently truthful speakers assign different probabilities to different sentences. Crucially, this allows speakers to be more informative to their listener by upweighting sentences carrying a lot of information about $w$ compared to other sentences. In linguistic pragmatics, RSA has been proposed as a mathematical account of such Gricean speakers \citep{goodman2016pragmatic}, and we show in \autoref{sec:rsa} that a conditionally-independent model of an RSA speaker is a special case of an independently truthful speaker. Thus, \autoref{cor:sta-cia} holds for RSA speakers with the simplifying assumption that different sentences are conditionally independent.

While independently truthful speakers are much more naturalistic than uniformly truthful speakers, and in some sense come close to modeling Gricean speakers, there is good reason to question the validity of the the conditional independence assumption.
Consider how, under conditional independence,
a sentence $y$ is likely to occur after $x$ even if $x$ entails $y$. Indeed, our distributional isomorphism for entailment relies on the probability $p(xy)$. In natural language, however, it is unnatural to produce sentences that contribute no information given what has already been said:
\begin{enumerate}
    \item John has at least two dogs. In fact, he has three.
    \item *John has at least two dogs. In fact, he has a dog.
\end{enumerate}
In the first text, the second sentence contributes new information given the first, and thus is pragmatically appropriate. In the second text, the second sentence is entailed by the first, and thus is strange to produce.
This shows the limits of the conditional independence assumption that is crucial to \autoref{thm:cia-sta}, and motivates our upcoming analysis of Gricean speakers in \autoref{sec:informative}.\footnote{While naturalistic text does not satisfy the conditional independence assumption, it could be possible to sample from LMs in a way that satisfies it approximately by conflating each world with a prompt. Specifically, two sentences $x,y$ could be sampled given the same prompt $w$, and then concatenated to form a text $xy$. Since $x,y$ would be conditionally independent, it is possible such texts would satisfy the isomorphism derived in \autoref{thm:cia-sta}.}

\section{Nonredundantly Truthful Speakers} \label{sec:nonredundant}

In \autoref{sec:informative}, we studied a class of speakers who aim to be informative to their listener. This was motivated by the idea that redundant text is unnatural, and Gricean speakers will avoid being redundant.
Here, we different class of \emph{nonredundantly truthful} speakers and derive a different distributional test for entailment.

\begin{definition}
A speaker $p(y \mid x, w)$ is nonredundantly truthful if
\begin{equation*}
    p(y \mid x, w) = 0 \iff \den{y}(w) = 0 \vee \den{xy} = \den{x} .
\end{equation*}
\end{definition}
All sentences generated by a nonredundantly truthful speaker will be true and will also avoid conveying the same information twice.
We will now show that this speaker assigns a zero probability to a document $xy$ if and only if $x,y$ are contradictory or $y$ is entailed by $x$:
\begin{lemma} \label{lem:nonredundant}
For any nonredundantly truthful speaker $p$,
\begin{equation*}
    p(xy) = 0 \iff \den{xy} = \emptyset \vee \den{x} \subseteq \den{y} .
\end{equation*}
\end{lemma}
\begin{proof}
The probability that $p$ assigns to $xy$ is
\begin{equation*}
    p(xy)
    = \sum_w p(x \mid \omega, w) p( y \mid x, w) ,
\end{equation*}
which is $0$ if and only if, for all $w$,
\begin{align*}
    p(x \mid \omega, w) p( y \mid x, w) &= 0 \\
    \den{x}(w) = 0 \vee \den{y}(w) &= 0 \vee \den{xy} = \den{x} .
\end{align*}
Since $\den{xy} = \den{x} \cap \den{y}$, this if and only if $\den{x} \subseteq \den{y}$, or, for all $w$,
\begin{equation*}
    \den{x}(w) = 0 \vee \den{y}(w) = 0 .
\end{equation*}
This letter condition is equivalent to saying that there is no world where $x,y$ are both true, i.e., $\den{xy} = \emptyset$.
\end{proof}

\autoref{lem:nonredundant} motivates a test for strict entailment between two propositions. Strict entailment is an assymetric version of entailment, i.e., $x$ strictly entails $y$ if $\den{x} \subset \den{y}$. With a nonredundantly truthful speaker, strict entailment is isomorphic to a distributional relation different than the one we found for entailment under the CIA:

\begin{theorem} \label{thm:nonredund}
For any nonredundantly truthful speaker $p$, strict entailment is isomorphic to a distributional relation $d_p(x, y)$. For any sentences $x,y \in \mathcal X$,
\begin{equation*}
    \den{x} \subset \den{y} \iff p(xy) = 0 \wedge p(yx) \neq 0 .
\end{equation*}
\end{theorem}
\begin{proof}
By \autoref{lem:nonredundant}, we know that $d_p(x, y)$ holds if and only if
\begin{align*}
    \left( \den{xy} = \emptyset \vee \den{x} \subseteq \den{y} \right) \wedge
    \left( \den{yx} \neq \emptyset \wedge \den{y} \not\subseteq \den{x} \right) .
\end{align*}
Intesecting these two formulae and simplifying, this is equivalent to
\begin{equation*}
    \den{x} \subseteq \den{y} \wedge \den{y} \not\subseteq \den{x} .
\end{equation*}
Thus, we can conclude that $d_p(x, y) \iff \den{x} \subset \den{y}$.
\end{proof}

\subsection{Discussion}

\autoref{thm:nonredund} shows that nonredundant speakers, even if they are not explicitly informative, admit a distributional test for entailment.
This is interesting because redundant texts were central to the proof construction for conditionally independent speakers, and still potentially receive nonzero probability from Gricean speakers. Here, we have shown that explicitly removing all redundancy still allows for a simple distributional relation to be derived.

That being said, this speaker model is likely less realistic than the Gricean speakers studied in \autoref{sec:informative}.
The assumption that redundant expressions get zero probability may be too strong: in practice, redundant expressions may have low, but nonzero probability, or even be likely in certain contexts. For example, dynamic RSA (cf. \autoref{sec:rsa}) assigns low, but nonzero, probability to redundant sentences. Thus, rather than enforcing that speakers are \emph{never} redundant, it makes makes more sense to analyze speakers who strive to be informative to their listener.
